# Supplementary material for: A Survey on Deep Learning for Human Mobility
Source: arXiv:2012.02825 source file (2021-06-27)
Supplement: Supplementary file 2 [file appendix_data.tex]

The last decade has witnessed the emergence of massive datasets of digital traces that portray human movements at an unprecedented scale and detail. 
Examples include tracks generated by GPS devices embedded in smartphones \cite{zheng2010geolife} or private vehicles \cite{pappalardo2013understanding}; 
mobile phone records  \cite{blondel2015survey}; and geotagged posts from social media platforms \cite{noulas2012tale}. 
Unfortunately, most of these datasets are proprietary and not publicly available, making research on human mobility hard to reproduce.
In this section, we discuss the peculiarities of various sources of mobility data. 
For each data source, we provide a reference to a list of datasets that are available for research (Table \ref{tab:open_datasets}).
We identify and discuss three primary data sources: mobile phone data (Section \ref{sec:mobile_phone_data}), GPS traces (Section \ref{sec:gps}), and social media data (Section \ref{sec:social_media}). 
Moreover, in Section \ref{sec:auxiliary} we discuss data sources that convey important auxiliary information (traffic, environmental, and census and administrative data). 

\subsection{Mobile Phone data} 
\label{sec:mobile_phone_data}
Nowadays, mobile phones are ubiquitous, with coverage in most countries that reaches almost 100\% of the population \cite{blondel2015survey, itu2019}. 
Telco companies record the activity of their users for billing and operational purposes, hence storing an enormous amount of information on where, when, and with whom users communicate \cite{blondel2015survey}. 

Every time a user engages a telecommunication interaction -- makes or receives a call or a text message, or uses the mobile data connection -- the operator assigns a Radio Base Station (RBS) to deliver the communication through the network. 
Since the position and the coverage area of each RBS are known, a user's telecommunication interaction reflects their geographic location.
Each telecommunication interaction generates several mobile data formats, the most used of which are Call Detail Records (CDRs) and eXtended Detail Records (XDRs) \cite{pappalardo2020individuallevel}. 

Every time a user makes/receives a call or sends/receives an SMS, a new Call Detail Record (CDR) is created recording the time of the interaction, the RBSs that handled it, and the two users' anonymized identifiers. 
A CDR is a tuple $(\mbox{u}_o, \mbox{u}_i, t, A_o, A_i, d)$, where $\mbox{u}_o$ and $\mbox{u}_i$ are the identifiers of the caller and the callee, respectively, and $t$ is a timestamp of when the call starts. 
In turn, $A_o$ and $A_i$ are the RBSs that manage the outgoing call and the receiving call, respectively, and $d$ is the call duration.  
An individual's mobility can be reconstructed from CDRs assuming a movement between the RBSs of any two consecutive records \cite{blondel2015survey}. 
Aggregated mobility, such as crowds' movements, can be inferred by counting the number of users that move, in a given time window, between two RBSs or spatial aggregations of them (e.g., neighborhoods or municipalities) \cite{calabrese2011estimating}.
CDRs are sparse in time, i.e., a user's position is known when they make or receive a call or a text message only, leading to sparse and incomplete mobility trajectories.  
Notwithstanding, CDRs are by far the most common format of mobile phone records, used for a large number of studies on human mobility \cite{gonzalez2008understanding, simini2012universal, csaji2013exploring, barbosa2015effect, pappalardo2015returners, blondel2015survey}.

When a user uploads or downloads data from the Internet using their phone's mobile connection, they generate an eXtended Detail Record (XDR), a tuple $(\mbox{u}, t, A, k)$ where $A$ is the RBS that serves the connection, and $k$ the amount of uploaded/downloaded information. XDRs are less common in the literature than CDRs, mainly because the advent of the mobile data connection is relatively recent. XDRs partially overcome the problem of sparsity present in CDRs \cite{chen2019complete}, because mobile connections are more frequent than calls and text messages.

For both CDRs and XDRs, the spatial granularity is at the level of RBS, i.e., the user position is approximated with the location of the RBS used for the telecommunication activity. 
This approximation implies that the user's position within an RBS's coverage area is unknown and that user tracking depends on the spatial distribution of antennas on the territory, which depends on population density. 
Nevertheless, mobile phone data may cover a large sample size on a national scale. 
An advantage of mobile phone data is its multidimensionality: CDRs also provide information about the social interactions between users; both CDRs and XDRs may be accompanied by socio-demographic information about the users (e.g., age, sex).  

\subsubsection{Available datasets.}
Since mobile phone data contain sensitive information \cite{pellungrini2017data, demontoye2018privacy}, they are not typically publicly available, and any data collected by a specific group of researchers may not be shared with other groups, making reproducibility difficult.
Some companies launched initiatives, e.g., data challenges, to release large scale CDRs for research upon requests, such as the Telecom Italia's Big Data Challenge (TBDC) \cite{barlacchi2015multi}. 

Nevertheless, some aggregated information extracted from mobile phone data has been publicly released in the last few years. 
For instance, the WorldPop project \cite{tatem2017worldpop} integrates mobile phone data with censuses, surveys, and other data sources to estimate the population density worldwide with a spatial granularity of 100m$\times$100m cells. 

The provided dataset is especially relevant for low-income and mid-income countries in which official surveys and census data may be inconsistent and with an inadequate spatial granularity \cite{tatem2014mapping}. 

Du et al. \cite{du2018temporal} make publicly available three datasets about the displacements of two million users in the Changchun over one week: 1) the temporal network, describing the last location visited by each user per each hour of the day; 2) the mobility network, describing the number of users moving between a pair of RBSs for every hour of the day; 3) a matrix of the distances between locations, since they do not provide a precise geographic position of the locations.
Similarly, Du et al. in \cite{du2019inter} provides, for one week, hourly aggregated movements of almost three million users among 167 administrative divisions in Sangliao Basin, northeast China ($\approx20$ km$^2$). 
 
TBDC \cite{barlacchi2015multi} publish three multi-source datasets containing mobile phone activities (aggregations of CDRs and XDRs) over two months in Milan and the Province of Trentino, Italy. 
The first dataset describes the incoming and outgoing calls/messages and internet traffic data activity for each cell of a squared tessellation. 
The second dataset depicts the interaction between the cells in Milan/Trentino and other Italian provinces. 
The third dataset provides the directional interaction strengths between pairs of cells in Milan and Trentino. 

Other mobility datasets are available on-site upon the approval of a project proposal. 
For example, the EU-funded research infrastructure SoBigData \cite{grossi2020data} opens regular calls for projects proposal on datasets of various types, including mobility ones \cite{andrienko2020sobigdata}. 
In particular, the SoBigData catalog \cite{sobigdata_catalogue} includes CDRs regarding Tuscany, the city of Pisa, and the city of Rome, Italy.

\subsection{GPS traces}
 \label{sec:gps}

Global Navigation Satellite Systems (GNSS) are an essential source of human mobility data.
A navigation satellite system uses satellites to provide geo-spatial positioning, allowing electronic receivers to determine their location (longitude, latitude, and altitude) and time, using signals transmitted along a line of sight from satellites. 
The US Global Positioning System (GPS), the Russian Global Navigation Satellite System (GLONASS), the Chinese BeiDou Navigation Satellite System (BDS) ad the EU Galileo are all examples of GNSS. 
Among these systems, GPS is by far the most popular one, and GPS receivers are ubiquitous in many tools of everyday life, such as mobile phones \cite{zheng2010geolife, stopczynski2014measuring, alessandretti2018evidence}, vehicles \cite{pappalardo2013understanding, pappalardo2015returners, gallotti2015stochastic}, vessels \cite{russo2016assessing, vespe2016mapping, Sleimani2015anomaly}, and wearable devices \cite{rossi2018effective}.
On mobile phones, the GPS receiver is activated by apps that require the user's position (e.g., Google Maps).
On vehicles, the GPS device automatically turns on when the vehicle starts, sending positions to a server with a frequency of a few seconds. 
The precision of GPS receivers varies from a few centimeters to meters, depending on the device's quality and the errors generated by the system \cite{Carlson-2010-10506}.
Moreover, GPS cannot track the devices in enclosed spaces, such as buildings and tunnels.
A typical GPS trace is a set of tuples $(u, t, lat, lng)$ where $u$ is a user, $t$ is a timestamp of the measurement and $lat, lng$ are the position's latitude and longitude. 
GPS traces may require several preprocessing tasks aimed to mitigate errors and extract meaningful semantics. 
For example, since GPS traces are dense sequences of spatio-temporal points, they do not explicitly define semantic locations, which must be inferred through specific preprocessing techniques \cite{feng2016survey,zheng2014urban, zheng2015trajectory}. 

\subsubsection{Available datasets}
GeoLife \cite{zheng2010geolife} is a publicly available dataset describing the GPS trajectories of 182 users over 4.5 years, collected using different devices (e.g., GPS receivers and mobile phones) every 1-5 seconds or 5-10 meters.
GeoLife covers a broad range of users' outdoor movements, from life routines like go home and go to work to entertainment and sports activities. 
Each point in a GeoLife's trajectory contains latitude, longitude, altitude, and the timestamp.
Moreover, the user's transportation mode is also available for most of the trajectories.

In 2013, OpenStreetMap (OSM) released a GPS dataset that contains information from seven years of activity, corresponding to almost three billion GPS points \cite{gps_osm}.
The dataset describes GPS trajectories, uploaded by voluntary users, which describe movements with different transportation means. 
The last updated version of the dataset dates back to April 2013, but it is possible to download more recent GPS traces using OSM's APIs.
%Despite the large amount of information in the dataset, almost one million points are located at position $(0,0)$, in the middle of the Pacific ocean, and refer to geolocation errors. 
The geographic distribution of GPS points is denser in specific countries and regions: 
%For example, the number of points located in Germany is higher than the number of all points in the Americas, Africa, Australia, and Asia. 
20\% of the world contains 75\% of the measurements. 
%Finally, particular care should be devoted to data cleaning. For example, the dataset contains GPS traces from crop-dusting airplanes that may introduce noise. 

Other public datasets provide information about the trips of GPS-equipped taxis in several cities. 
Piorkowski et al. \cite{epfl-mobility-20090224} provide the trajectories, sampled on average every 10 seconds, of taxis in San Francisco, in May 2008. 
Each point of a trajectory consists of the taxi's identifier, the latitude, the longitude, the timestamp, and the occupancy. 
Bracciale et al. \cite{roma-taxi-20140717} provide trajectories of taxis in Rome, Italy, in which points are gathered on average every 7 seconds. 
Each point contains the taxi's identifier, the latitude, the longitude, and the timestamp. 
Moreira et al. \cite{moreira2013predicting} (ECML/PKDD Challenge) provide the trips of taxis in Porto, Portugal, in which points contain the latitude, the longitude and a timestamp indicating when the trip started. Data are collected approximately every 15 seconds.  
For each trip, the dataset provides several auxiliary information, such as the trip's typology (e.g., dispatched from the central, demanded to the operator, requested to the driver), the stand from which the taxi departed, and an identifier of the passenger's phone number. 
The Taxi and Limousine Commission of New York City collected a dataset on yellow and green taxis operating in the city starting from 2009 \cite{tlc}. The dataset provides information on pick-up and drop-off dates/times and locations, trip distances, itemized fares, rate types, payment types, and driver-reported passenger counts.

The T-Drive dataset \cite{zheng2011t-drive}  describes the trajectories of about 10,000 taxis in Beijing, China, for one week.
Points are sampled every 177 seconds and contain the taxi's identifier, the latitude, the longitude, and the timestamp. 
%Microsoft's team also provided an aggregated version of such information in \cite{zhang2017deep}. In particular,
Zhang et al. \cite{zhang2017deep} create a squared tessellation on New York City and Beijing and, for each tile, provide the incoming and the outgoing flows. 
Beijing's flows are captured based on taxis' GPS signal; the New York City ones are based on the city's bike-sharing system. 

Citi Bike by Lyft \cite{bikenyc} provides a dataset describing the trips between bike-sharing stations in New York City. 
Each record describes the stations where the trip started and ended when it took place and the stations' coordinates. 
There are similar open datasets for other cities, such as Washington DC \cite{bikewo}.

The Mobile Data Challenge dataset (MDC) \cite{laurila2012mobile} describes the trajectories of 185 participants of the Lausanne Data Collection Campaign, collected from mobile phones  \cite{kiukkonen2010towards}.
The dataset offers various information (e.g., calendar logs and data from accelerometers), including two files describing the individuals' mobility through GPS receivers and Wireless Local Area Networks (WLANs). 
Each record in the file with the GPS tracks describes the user's identifier, latitude, longitude, altitude, timestamp, speed, heading direction, and accuracy. 
The WLANs file provides a set of records describing the user's identifier, a timestamp, the first three bytes of the device's MAC address, and the access points' location. 

Other GPS datasets are available on-site upon the approval of a project proposal, such as tracks of private vehicles and traces provided by voluntary individuals traveling in Italy, provided by SoBigData \cite{sobigdata_catalogue, andrienko2020sobigdata}.

Recently, to take countermeasures for the COVID-19 pandemic, companies such as Cuebiq and SafeGraph are providing free access upon request to their data.\footnote{Cuebiq: \href{https://www.cuebiq.com/visitation-insights-covid19/}{cuebiq.com/visitation-insights-covid19/}, SafeGraph: \href{https://www.safegraph.com/covid-19-data-consortium}{safegraph.com/covid-19-data-consortium}} 
The former allows researchers to access mobility insights such as traveler analysis, home switcher trend, and a mobility dashboard. SafeGraph allows for accessing three datasets: the first two contain information about points of interest (POIs), e.g., name, category, geometry, the third one about traffic patterns, e.g., how often people visit a place, how long they stay, where they came from.

\subsection{Social Media Data}
\label{sec:social_media}

Nowadays, users' posts on social media (e.g., photos, text, videos) can be geotagged, i.e., associated with a geographic location and time.
The presence of spatial and temporal information allows the reconstruction of users' trajectories from the sequence of published posts. 
Some platforms like Twitter provide two geotagging formats: the post's precise geotag (i.e., a latitude and longitude pair, a format recently removed) or the position of a predefined location suggested by the platform (e.g., a city, an area, a restaurant). 
In other platforms like Foursquare and Facebook, users can check-in in predefined locations called venues, i.e., POIs that provide information about social, cultural, and infrastructural components of a geographic area (e.g., cities, shops, museums).
A venue is associated with a physical location (latitude and longitude pair) and textual information (a description of the place or the activities related to the place) and can follow a hierarchical categorization that provides different levels of detail about the activities (e.g., Food, Asian Restaurant, Chinese Restaurant) \cite{barlacchi2017structural}. 
In Yelp, whenever a user publishes a comment or a photo, they can associate it with a specific geolocated business (e.g., restaurant). 
Similarly, Flickr users can post and geotag photos, which may be associated with predefined locations as well as specific coordinates.
In general, a geotagged record describes the posting user's identifier, the resource identifier (e.g., post, tweet, photo), the time of posting, and, depending on the platform, the venue identifier/category or a location as a string (e.g., Statue of Liberty, New York) or a latitude and longitude pair.
 
For most of the social media platforms, geotagged posts are downloadable through their APIs. 
APIs impose limitations on the number of downloadable posts and queries per day or require authorization from the platform's users to download the data.
Users' location is available only when they post something or check-in into a venue, leading to a data sparsity problem. 
Nevertheless, social media data bring the advantage that an objective definition of location is available, facilitating the data preprocessing phase \cite{cui2018social}.

\subsubsection{Available datasets}
Datasets about check-ins on social media platforms that are not active anymore, such as Gowalla and Brightkite, are freely available. 
Gowalla was a location-based social network platform in which, similarly to Foursquare, the users were allowed to check-in in the so-called spots (venues) through a website or the app. 
The related dataset \cite{cho2011friendship} consists of more than six million check-ins over one year and a half from February 2009 to October 2010. 
Each check-in describes the user identifier, the location identifier, the latitude and longitude pair, and a timestamp. 
The dataset also provides information about the users' friendship network, which contains about 200,000 nodes and one million edges \cite{cho2011friendship}. 
In Brightkite, another platform that is not active anymore, users were allowed to check-in in POIs, to specify who is nearby at the moment and who went to a POI before. 
The dataset contains almost 4.5 million check-ins from April 2008 to October 2010 and the users' friendship network with about 60,000 nodes and 220,000 edges \cite{cho2011friendship}. 

Yang et al. \cite{yang2014modeling} provide a Foursquare dataset collected over ten months and containing about 230,000 check-ins in New York City and 575,000 in Tokyo.
%(Figure \ref{fig:foursquare_checkins}).
Each check-in record describes the user's identifier, the venue's identifier and its category, latitude, longitude, and timestamp. 
Additionally, the same authors also collected check-ins on a global scale from April  2012 to September 2013, involving 415 cities in 77 countries \cite{yang2015nationtelescope, yang2015participatory}. 
This dataset also provides the country code of the venue and information on the 415 cities involved in the study (latitude, longitude, country code and name, type of city). 
They also offer the possibility to associate, for about 18,000 users in New York City and 12,000 in Tokyo, with the related gender, the number of following and follower users on Twitter \cite{yang2016privcheck}. 
Another dataset collected through Foursquare APIs is introduced in \cite{feng2018deepmove} and contains check-ins of 16,000 users over one year in New York City.

The Yahoo Flickr Creative Commons 100 Million Dataset (YFCC100M) \cite{Thomee_2016} contains 100 million open-license media objects (photos and videos) collected between 2004 and 2014 from the popular service Flickr. 
Each record describes the camera's model used to take the photo or video, a set of tags, and the timestamp when the photo or video was made. 
For about 48 million photos and 100,000 videos, the geographic location is also available as latitude and longitude pair, either inserted manually by the user or through the device's GPS receiver. 

Twitter provides several open datasets, in which location is usually expressed as a semantic point of interest either suggested by the platform (e.g., Empire State Building, NYC) or typed by the users (e.g., Home), or as a latitude and longitude pair. 
Geotagged tweets may be retrieved directly using Twitter APIs.
For example, Zhang et al. \cite{zhang2016gmove} (GMove) provide a Twitter dataset describing 1.4 million tweets from August to November 2014 covering the area of Los Angeles. 
%Cheng et al. \cite{cheng2010you} collected almost 22.5 million tweets (72\% of which with a location) for about 1 million users in the United States. 
In 2020, some Twitter datasets with geotagged information have been released to track the COVID-19 pandemic \cite{geocov19, feng2020working}. 
A comprehensive list of Twitter datasets is available at \href{https://github.com/shaypal5/awesome-twitter-data}{github.com/shaypal5/awesome-twitter-data}.
%\footnote{Not all the datasets listed contains geotagged information}

Yelp released two datasets containing information about check-ins in 174,000 businesses for 11 metropolitan areas over four countries \cite{yelp}.
One dataset describes the geographic position of Yelp businesses, the other one describes the check-ins, each associated with a business identifier and timestamp but without the user's identifier that generated it. 

\begin{table}[]
    \scriptsize
    \begin{tabularx}{\textwidth}{c c X r c X X X}
      \toprule
      & \scriptsize \textbf{Ref.}   &   \scriptsize \textbf{Name}       &   \scriptsize \textbf{Items} &   \scriptsize \textbf{Time span}   &   \scriptsize \textbf{Area}     &   \scriptsize \textbf{Access} &   \scriptsize \textbf{Link (https://bit.ly/)} \\ \midrule 
    
      \multirow{4}{*}{\rotatebox[origin=c]{90}{\bf Phone}} & \cite{barlacchi2015multi}  &   TBDC              &        -                        &              2 months           &   Milan \& Trento, Italy                                             &   public  & \href{https://bit.ly/TBDC-2}{TBCD-2} \\
        
           %\cite{}  &    --------            &        -                        &           &                           &   public  &  \\
        
       & \cite{tatem2017worldpop}          &   WorldPop                        &         -                       &              20 years          &   World                                             &   public & \href{https://bit.ly/WorldPop-Data}{WorldPop-Data} \\
    
       & \cite{du2018temporal}          &   Changchun                            &         2M                       &               1 week          &   Changchun, China                                             &  public & \href{https://bit.ly/Changchun-Data}{Changchun-Data} \\
    
    & \cite{du2019inter}          &   Songliao Basin                            &         3M                       &               1 week          &   Sangliao Basin, China                                             &   public & \href{https://bit.ly/Songliao}{Songliao}\\
    
     \midrule
    
      \multirow{10}{*}{\rotatebox[origin=c]{90}{\bf GPS}} & \cite{zheng2010geolife}          &   GeoLife                                                             &    182                             &   4.5 Years                         &   Asia                                           &   public & \href{https://bit.ly/Geolife}{Geolife} \\ % \footnote{https://www.microsoft.com/en-us/download/confirmation.aspx?id=52367} &   \cite{al2016stf, wang2019statistics, zhang2019multi, wang2019exploring, zhou2019context}  \\
       
       & \cite{zheng2011t-drive}  &   T-Drive & 10k  &   1 Week  &   Beijing, China  &   public & \href{https://bit.ly/T-Drive-Data}{T-Drive-Data} \\ 
       %  \footnote{https://www.microsoft.com/en-us/research/publication/t-drive-trajectory-data-sample/}   &   \cite{zhang2018predicting, wang2019star}  \\
       
       & \cite{gps_osm} &   OSM & - &  7 years & World &   public & \href{https://bit.ly/osm_gps}{osm\_gps} \\

        & \cite{zhang2017deep} &   ST-ResNet taxis & - & 4, 6 months & Beijing, China & public & \href{https://bit.ly/ST-ResNet}{ST-ResNet}\\
       
       & \cite{zhang2017deep} &   ST-ResNet bikes & - & 6 months & New York City, USA & public & \href{https://bit.ly/ST-ResNet}{ST-ResNet}\\
    
       & \cite{epfl-mobility-20090224} & Taxi San Francisco  & 500 & 30 days & San Francisco, USA  & upon registration & \href{https://bit.ly/TaxiSF}{TaxiSF} \\ % \footnote{https://crawdad.org/epfl/mobility/20090224/ } & \cite{rossi2019modelling} \\ 
    
       & \cite{roma-taxi-20140717} & Taxi Rome & 320 & 1 months &   Rome, Italy & upon registration & \href{https://bit.ly/TaxiRome}{TaxiRome}  \\ %  \footnote{https://crawdad.org/roma/taxi/20140717/}     &      \\
       
       & \cite{moreira2013predicting}                          &   ECML-PKDD taxi  & 441 & 9 months & Porto, Portugal  & public & \href{https://bit.ly/TaxiPorto}{TaxiPorto} \\ % \footnote{https://www.kaggle.com/c/pkdd-15-predict-taxi-service-trajectory-i/data}   &   \cite{rossi2019modelling} \\ 
    
       %\cite{mokhtar2017priva}          &   Priva'Mov                                                        &    100                             &   15 Months                       &   Lyon, France                                        &   Upon Request \\ % \footnote{https://projet.liris.cnrs.fr/privamov/project/dataset}    &   \\ 
       
       & \cite{tlc} & Taxi New York City & - & From 2009 & New York City & public & \href{https://bit.ly/TaxiNYC-2}{TaxiNYC-2} \\ 
       
       %\cite{sobigdata_catalogue} & Tuscany vehicles & 150k & 1 month & Tuscany, Italy & on-site & \href{https://bit.ly/GPSTuscany}{GPSTuscany}\\
       
       %\cite{sobigdata_catalogue} & Calabria vehicles & 115k & 2 Months & Calabria, Italy & on-site & \href{https://bit.ly/GPSCalabria}{GPSCalabria}\\
       
       %\cite{sobigdata_catalogue} & volunteers' tracks & - & 4 months & Tuscany, Italy & on-site & \href{https://bit.ly/VolunteersTrack}{VolunteersTrack} \\
       
       & \cite{laurila2012mobile} & MDC & 185 & 2 years &   Lausanne, Switzerland & upon request & \href{https://bit.ly/MDC-2}{MDC-2} \\ 
        %\cite{cabrero2015understanding} & Asturias emergency & - & 1 year & Oviedo, Spain & upon registration & \href{https://bit.ly/asturies-er}{asturies-er} \\
    
       %\cite{rio_bus}  &   Rio Buses &  12k & 1 month &   Rio de Janeiro, Brazil & upon registration & \href{https://bit.ly/RioBusData}{RioBusData} \\
    
       %\cite{ves_1} &  Vessels  & - & 1 month &   Mediterranean Sea &  public &  \href{https://bit.ly/sea-data}{sea-data}\\
    
       %\cite{apple_covid}   &   Apple report   &   -     &  from Jan 2020 & World & public & \href{https://bit.ly/AppleMobility}{AppleMobility} \\
    
       %\cite{google_covid}   &   Google report  & - & from Jan 2020 &   World & public & \href{https://bit.ly/GoogleMobility2}{GoogleMobility-2} \\
    
        %\cite{}   &  Cuebiq  &  &  & &  \\
         
        %\cite{}   & SafeGraph  &  &  &  &  & \\
    
      %\midrule 
      %\multicolumn{7}{c}{\textbf{Social Media Data}} \\ 
      \midrule
    
      \multirow{9}{*}{\rotatebox[origin=c]{90}{\bf Social Media \& checkins}} &  \cite{cho2011friendship}         &   Gowalla &    196k   &   20 months  &   California \& Nevada, USA   & public & \href{https://bit.ly/GowallaData}{GowallaData} \\ %  \footnote{http://snap.stanford.edu/data/loc-Gowalla.html} & \cite{feng2017poi2vec, liu2020exploiting, feng2017poi2vec, zhang2020next, liudapred, yang2017bridging, yang2017neural, gao2019predicting, altaf2018spatio, liao2018multi, liu2016predicting, liu2020exploiting, feng2017poi2vec, zhang2020next} \\ 

      &  \cite{cho2011friendship}         &   Brightkite   &  58k  &   30 months  & - & public & \href{https://bit.ly/Brightkite}{Brightkite}  \\ % \footnote{http://snap.stanford.edu/data/loc-Brightkite.html} & \cite{yang2017neural, altaf2018spatio} \\

      &  \cite{yang2014modeling}  & Foursquare  &    800k          &   10 months  & NYC, Tokyo, World & public  & \href{https://bit.ly/Foursquare-Data}{Foursquare-Data} \\ %  \footnote{https://sites.google.com/site/yangdingqi/home/foursquare-dataset} & \cite{gao2019predicting} \\

      &    \cite{feng2018deepmove}       &   DeepMove    &   16k     & 1 Year      &  New York City  & public  & \href{https://bit.ly/DeepMove}{DeepMove} \\ % 
    
        % ====================
        % 47, 48 
        % ====================

       & \cite{yelp}  & Yelp &  200k  &   -   &   4 countries  & upon registration & \href{https://bit.ly/YelpData}{YelpData} \\ %  \footnote{https://www.yelp.com/dataset} &   \cite{yang2017bridging, liu2020exploiting}     \\     

    &    \cite{Thomee_2016}         &   YFCC100M    &    100M     &   10 Years     & World  & upon request &
        \href{https://bit.ly/YFCC100M}{YFCC100M}\\ %  \footnote{https://yahooresearch.tumblr.com/post/89783581601/one-hundred-million-creative-commons-flickr-images
       %} & \cite{gao2019predicting} \\
       
         %\cite{face_data}         &   RPC    &    100k     &   -     & -  & public & \href{https://bit.ly/rpc-data}{rpc-data}\\ %
         
         %\cite{}         &   facebook covid    &     &        &   &  & \\ %
    
       % \cite{yuan2013time}                          &   Foursquare Singapore                          &   Foursquare                     &                   &            &               &           & Available \\ %  \footnote{https://www.ntu.edu.sg/home/gaocong/datacode.htm}              &   \cite{feng2017poi2vec} \\

     &    \cite{zhang2016gmove}       &   GMove    &    1.4M    &   4 Months    & Los Angeles  & public & \href{https://bit.ly/SERM-Repo}{SERM-Repo} \\ % 
     
     &    \cite{geocov19}       &   GeoCoV19    &    43M    &   90 Days    & World & public & \href{https://bit.ly/GeoCoV19}{GeoCoV19} \\ % 

      & \cite{bikenyc}                   &   New York City bikes   &  -  & from 2013 &   New York City, USA &   public & \href{https://bit.ly/BikeNYCData}{BikeNYCData} \\

      & \cite{bikewo}  &   Washington DC bikes  & - & from 2010 &   Washington DC , USA  & public & \href{https://bit.ly/BikeWashington}{BikeWashington} \\

       % \multicolumn{7}{c}{\textbf{Auxiliary Data}} \\ 
       \midrule

      \multirow{6}{*}{\rotatebox[origin=c]{90}{\bf Auxiliary}} & -  &   Open Transport Map  & - & - &   World  & public & \href{https://bit.ly/OTM-DATA}{OTM-DATA} \\
        
     &    -  &   World Meteo. Org.  & - & - &   World  & public & \href{https://bit.ly/WMO-Data}{WMO-DATA} \\
        
      &  -  &   Weather Underground  & - & - &   World  & public & \href{https://bit.ly/WUnderground}{WUnderground} \\
        
       & -  &   EU Statistics & - & - &   European Union  & public & \href{https://bit.ly/EUCensusUB}{EUCensusUB}, \href{https://bit.ly/EUDataPortal}{EUDataPortal},\href{https://bit.ly/EUUrbasnAtlas}{EUUrbasnAtlas} \\
        
    &    - &   UN Statistics & - & - &   World  & public & \href{https://bit.ly/UNCensusHub}{UNCensusHub}\\
        
     &   -  &   OECD  & - & - &  World  & public & \href{https://bit.ly/OECDCensusHub}{OECDCensusHub} \\

       \bottomrule

    \end{tabularx} 
    \caption{Mobility datasets available for research. 
    For each dataset, we provide a reference to the paper introducing it, the number of items (users or points) in the dataset (symbol ``-'' indicates that the dataset is aggregated or that the number is not available), its time span, area covered, and access type (public, upon registration, upon request), and the link to download it.}
     \label{tab:open_datasets}
\end{table}

\subsection{Auxiliary Data}
\label{sec:auxiliary}

To add semantic to human mobility, deep learning models often use data describing the context in which movements take place. 
These auxiliary data may represent vehicular traffic, weather conditions, and census and administrative data. 
In what follows, we discuss these data's characteristics and summarize some data sources in Table \ref{tab:open_datasets}.

\subsubsection{Traffic data}

Sensors provide various information about urban traffic (e.g., the number of vehicles on the streets, their average speed) at various temporal aggregations. 
For example, cities like Turin, Italy Hamburg, Germany and New York City, US, have open datasets containing traffic information with temporal scales varying from minutes to days. 
The Open Transport Map project allows routing and visualization of traffic volumes in the EU. In general, traffic records contain a timestamp of the measurement and the number of vehicles, bikes, or pedestrians passed through a road segment between two consecutive measurements.  

\subsubsection{Environmental data}

Weather data are often used in crowd flow prediction because the meteorological conditions significantly impact how people move.
There are many datasets on the open data portals of regions, states and municipalities regarding the meteorological conditions, and there are also repositories that offer a global-scale perspective. In particular, the World Meteorological Organization allows downloading the forecast and climatologist information for almost all the nations.  
Weather Underground is a popular tool to retrieve temperature, dew point, humidity, wind speed, pressure, precipitation and weather conditions on a global scale, offering the possibility to explore different periods depending on the station and the city of interest. 

\subsubsection{Census and Administrative Data}

Census data provide information about the mobility flows, the socio-demographic characteristics, and the socio-economic status of a geographic region at various spatial scales \cite{barbosa2018human, voukelatou2020measuring}. 
They are periodically collected through surveys by public institutions and statistical bureaus every five or ten years and provide information about households' workplace, current and previous residence, and household members.
Census and administrative data are available from the websites of the national and international public entities and statistical bureaus responsible for the data collection and processing. 
The UN and the OECD provide portals with census data at national and international levels.
For a list of available census data sources and detailed discussions on how they are used for human mobility studies, the reader may refer to \cite{barbosa2018human, wang2019urban} and to the website of the UN statistics division\footnote{\url{https://unstats.un.org/home/nso_sites/}} and the OECD\footnote{\url{https://stats.oecd.org/}}.
For example, USCB collects data on commuting trips between counties in the US, in companion with further information on counties' spatial distribution and socio-demographic data.
Similarly, ONS collects commuting and migration flow for the UK at different spatial resolutions, and the EU CensusHub portal provides census data of all EU countries.
When not available on an open portal, commuting data are available to researchers on request from national statistics institutes.
Census data portals often contain land use data, which indicate the use class of each urban zone in a region, e.g., residential, commercial, and manufacturing. 
In this regard, the Urban Atlas on the EU Open Data Portal contains land use data standardized in 20 land use classes, covering cities of $100,000$ inhabitants or more.
